# Supplementary material for: Learning To Optimize Quantum Neural Network Without Gradients
Source: arXiv:2304.07442 source file (2023-04-15)
Supplement: Supplementary file 1 [file supplementary.tex]

\appendix
\onecolumn
\section{Supplementary Material: Further Ablation Experiments}

We will now present the results from ablation studies for our proposed method. We will focus on various different schemes for initializing the parameters for the meta optimizer and their effect on our algorithm. We will further focus on seeing the difference between the initialization with and without having a learned initial hidden state.

\begin{figure*}[t]
    \centering
    \begin{subfigure}[t]{.3\textwidth}
     \centering
     \includegraphics[width=\textwidth]{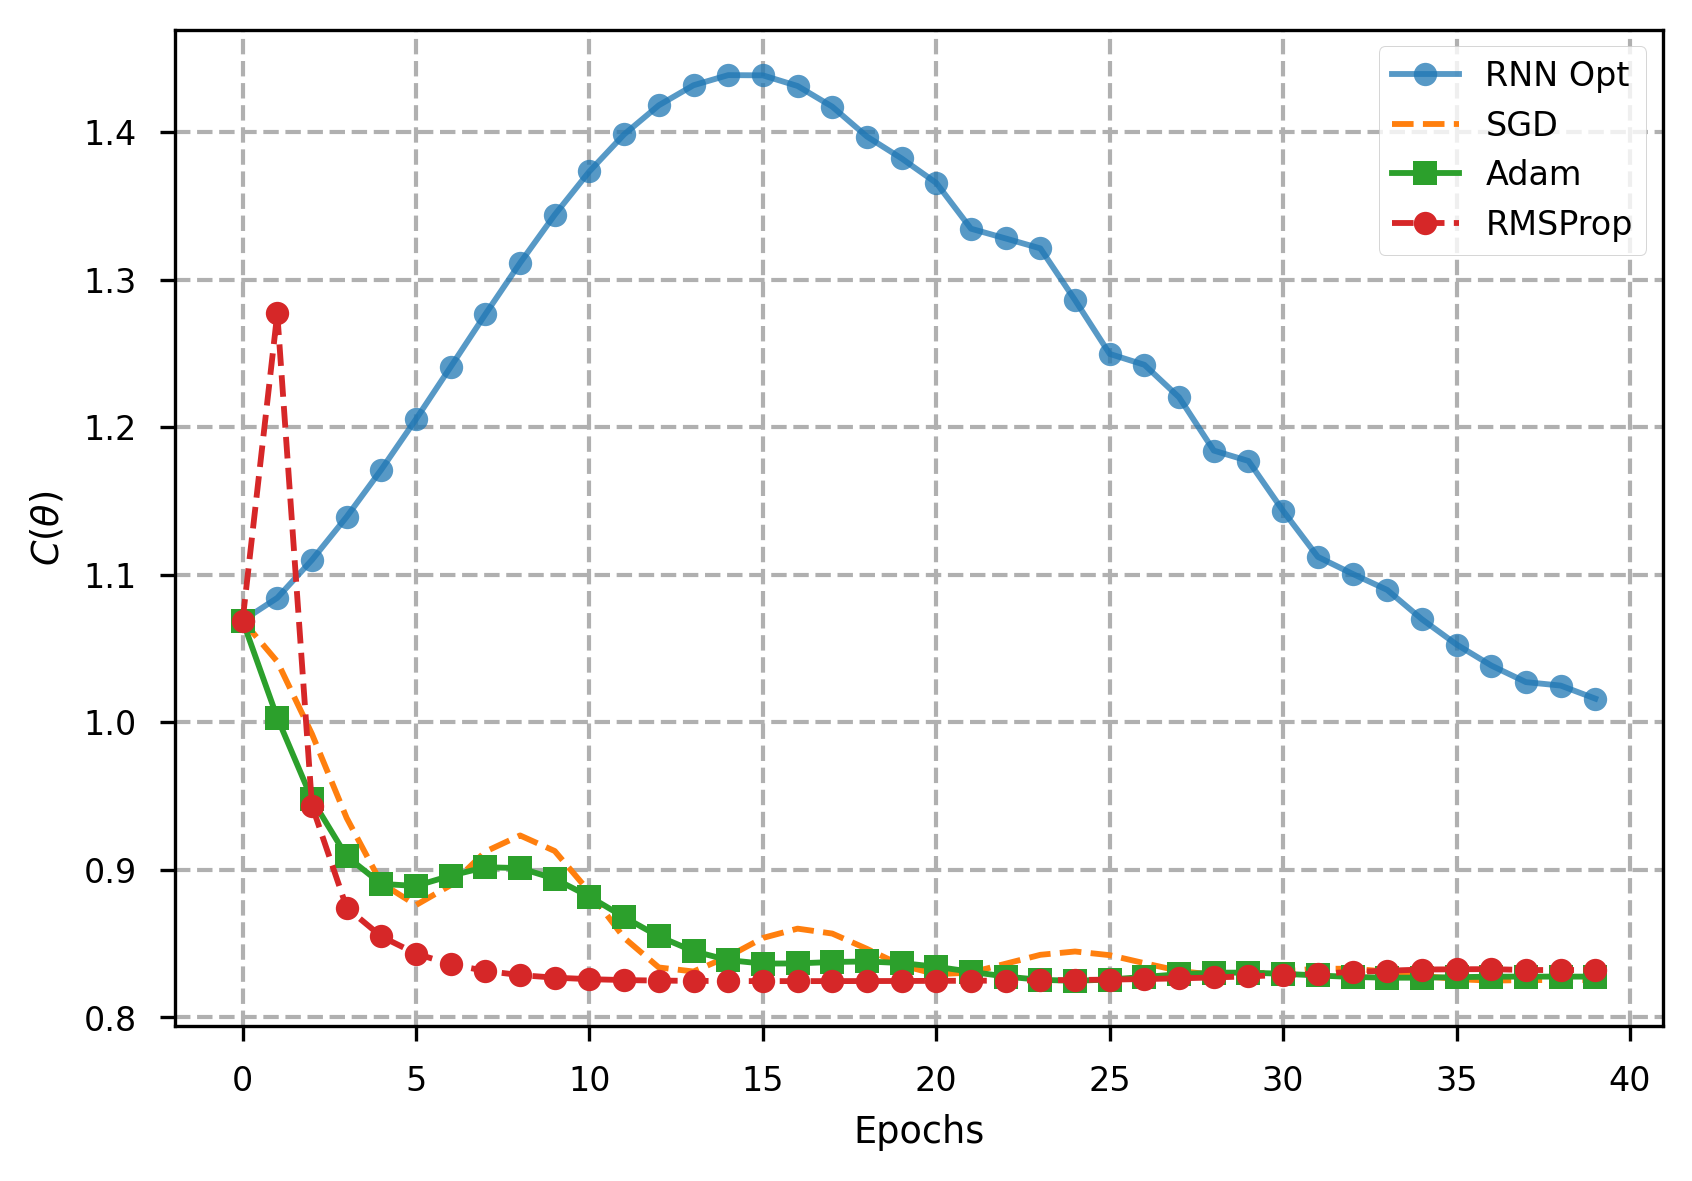}
    \caption{Iris - Zero Initialization}
    \end{subfigure}
    \begin{subfigure}[t]{.3\textwidth}
     \centering
     \includegraphics[width=\textwidth]{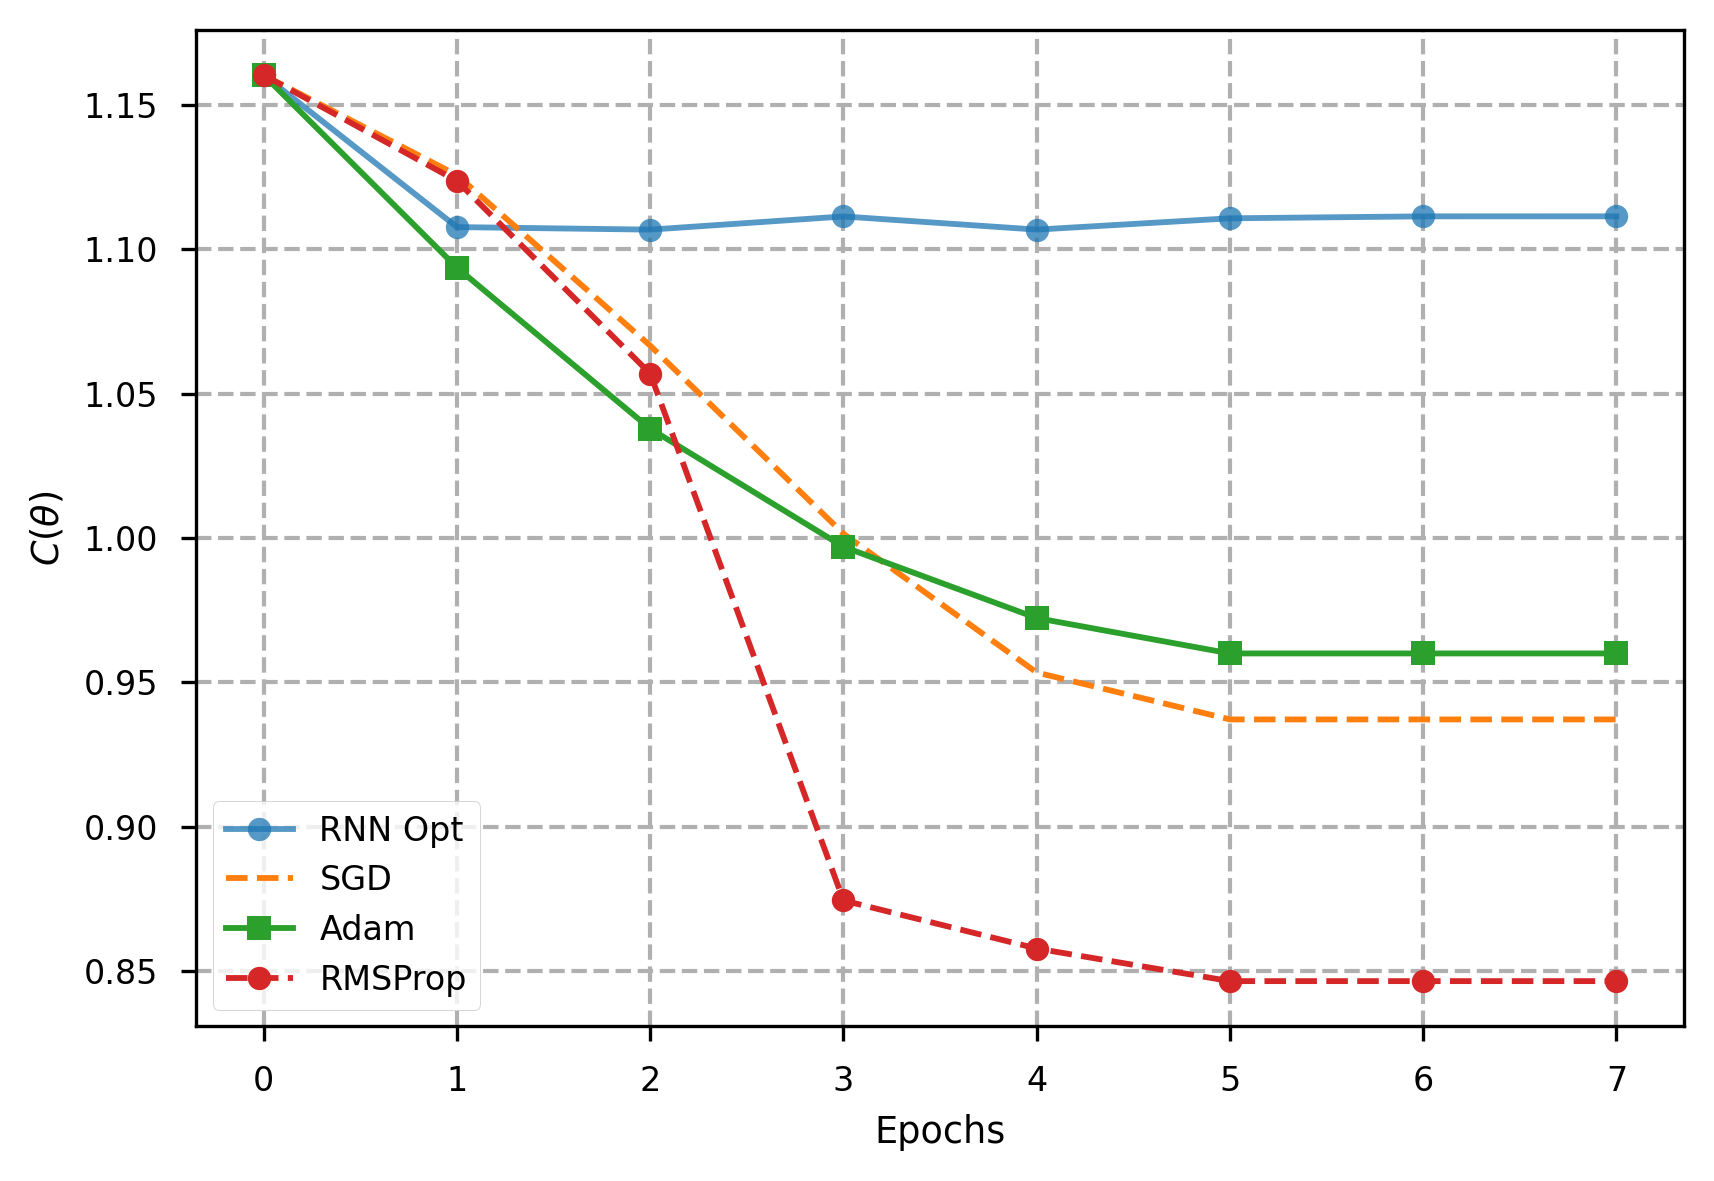}
    \caption{Iris - Uniform Initialization}
    \end{subfigure}

    \begin{subfigure}[t]{.3\textwidth}
     \centering
     \includegraphics[width=\textwidth]{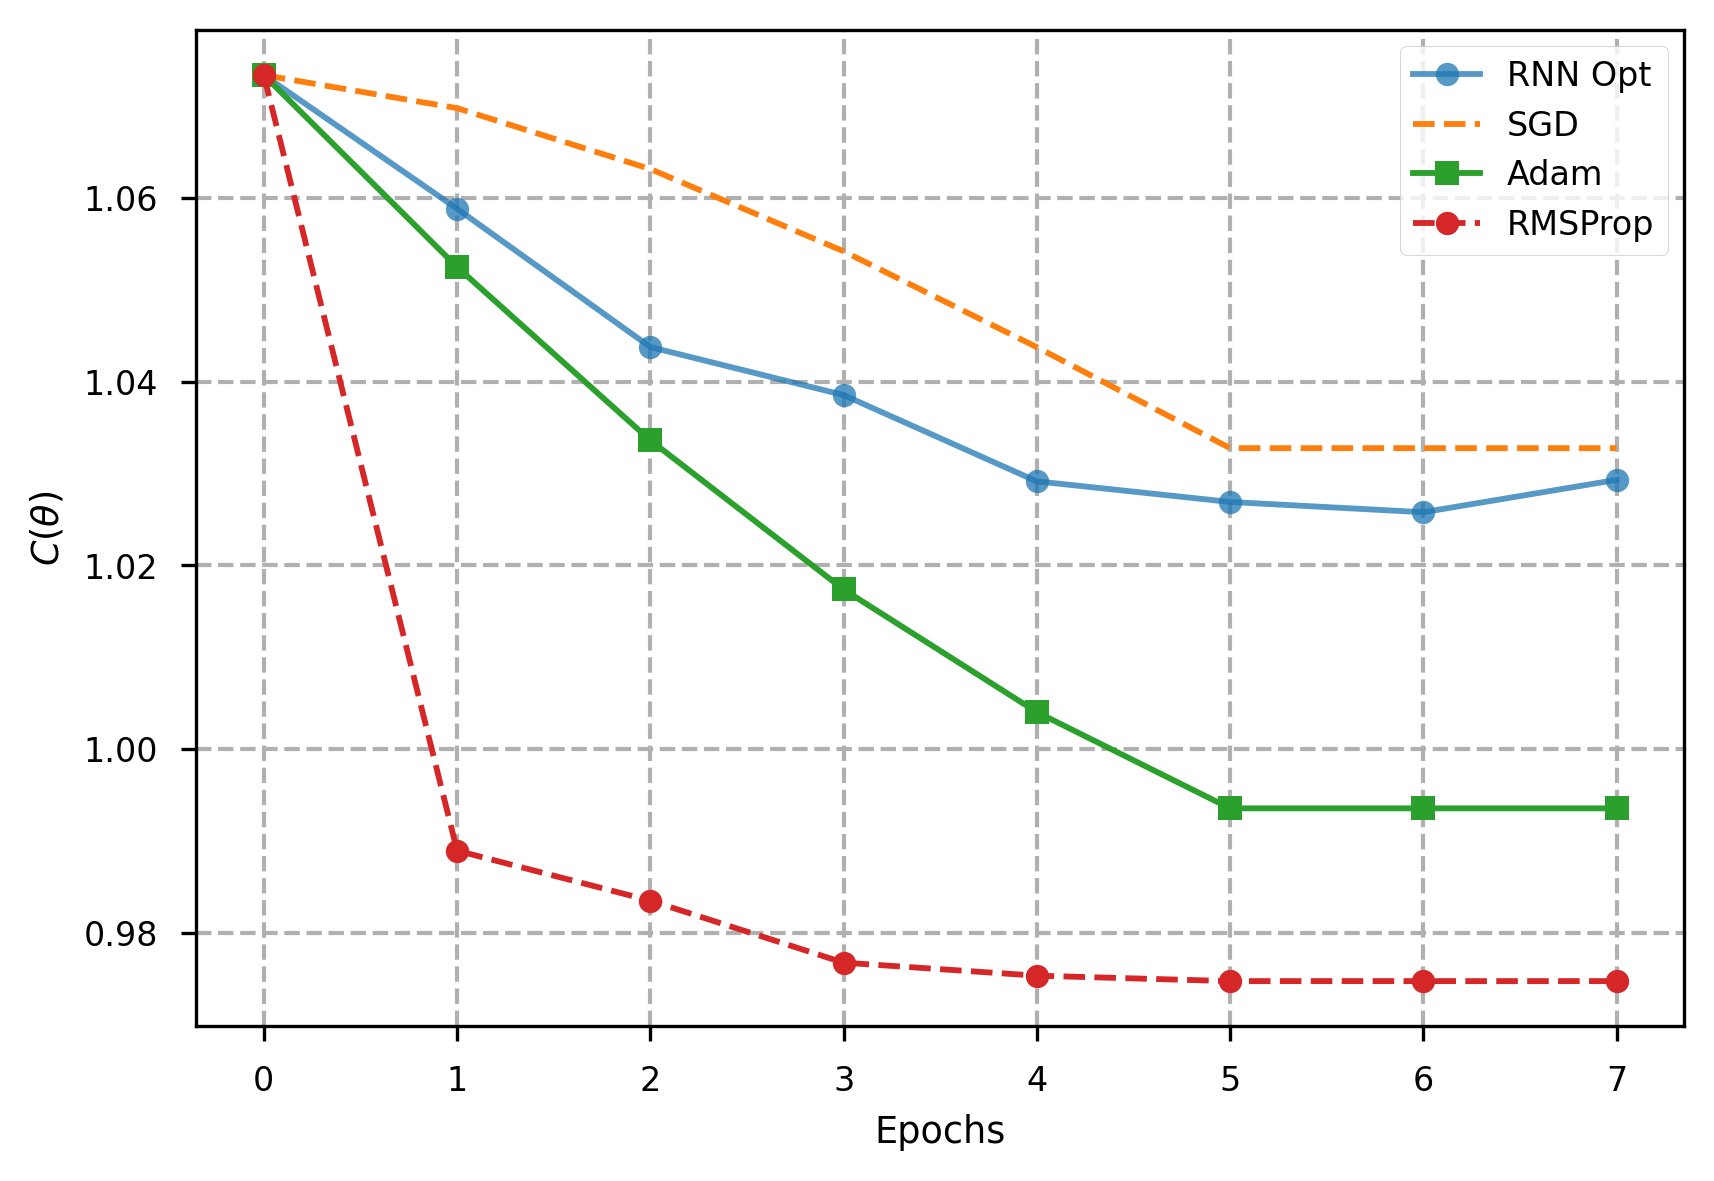}
    \caption{Gaussian - Zero Initialization}
    \end{subfigure}
    \begin{subfigure}[t]{.3\textwidth}
     \centering
     \includegraphics[width=\textwidth]{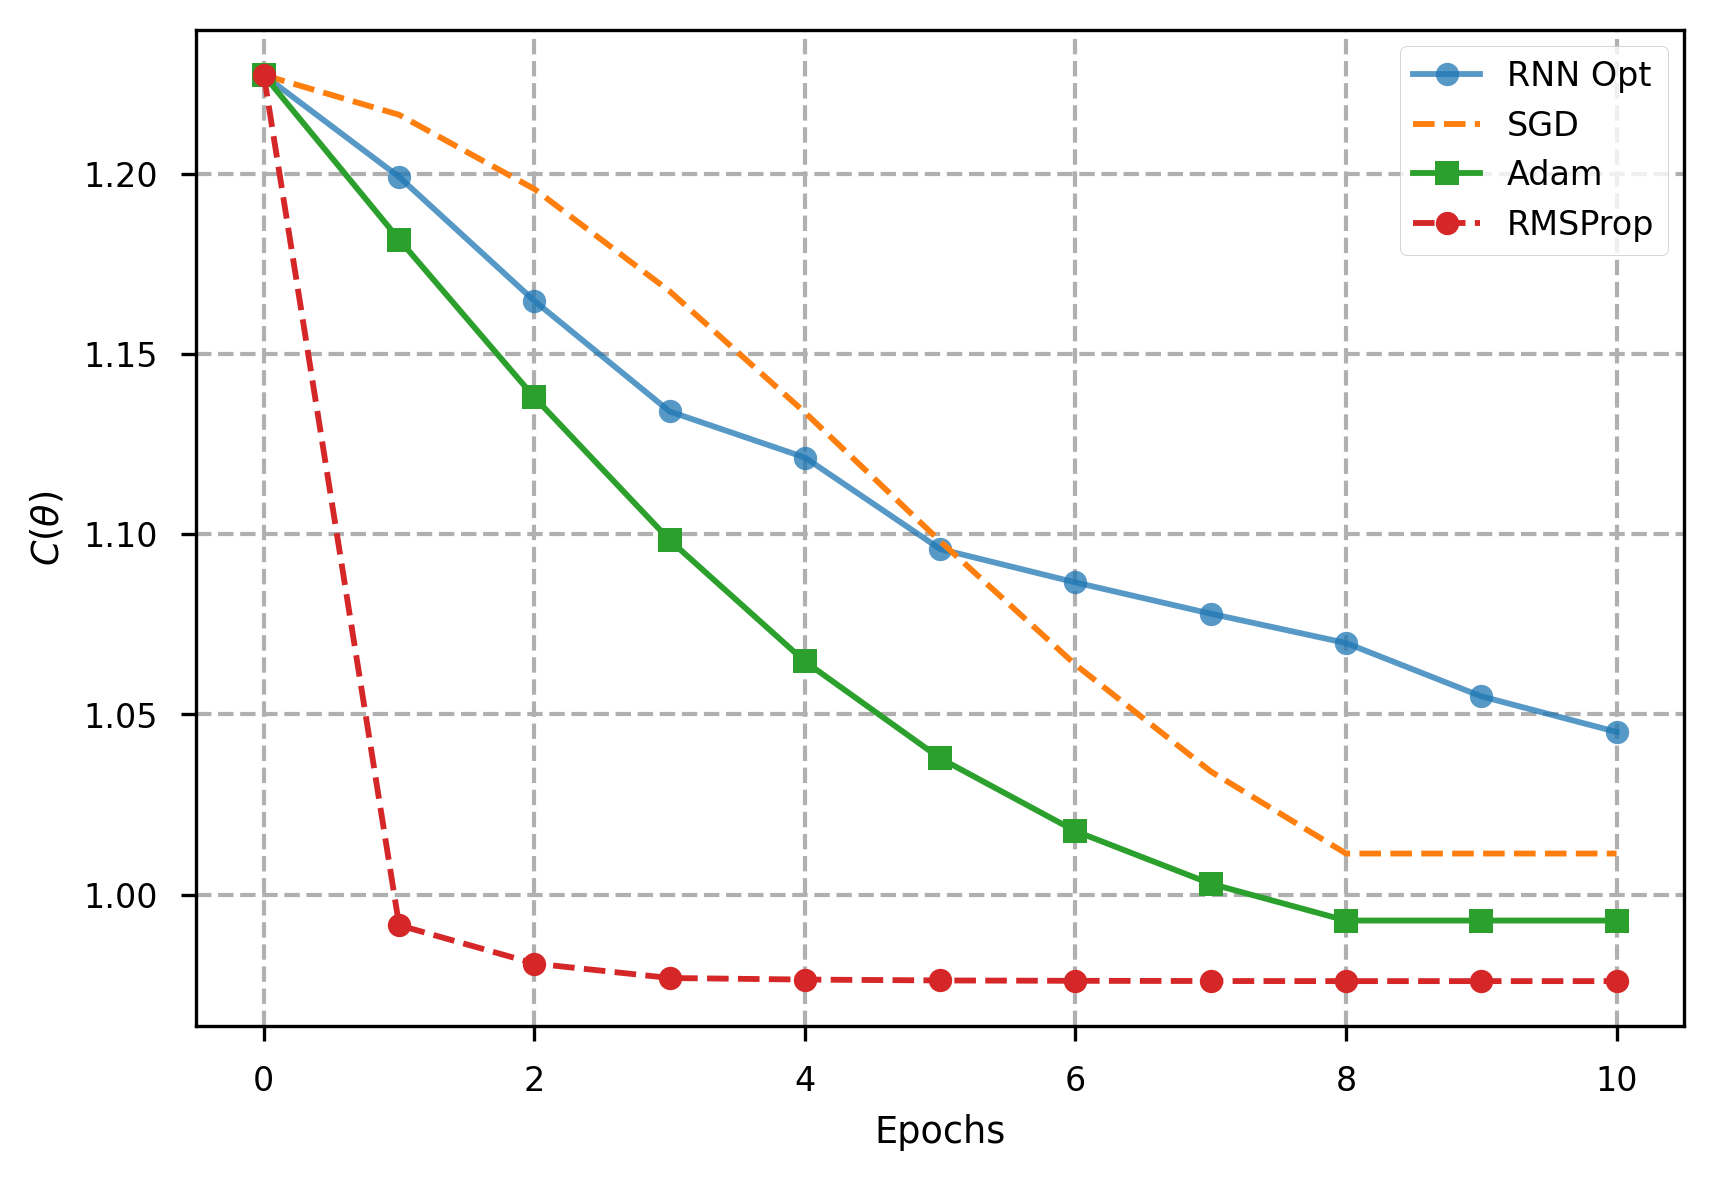}
    \caption{Gaussian - Uniform Initialization}
    \end{subfigure}
    \caption{Effect of meta-optimizer hidden state initialization with different initial distributions.}
    \label{fig:ablation_hidden_state_init}
\end{figure*}

\subsection{Dataset Description}
\label{ssec:sup-dd}

In this work, we have experimented with three different datasets - Iris, Gaussian and Spirals. The Iris dataset is a modified version of the original Iris dataset~\cite{dua2019} while the other two are synthetic datasets that are generated programmatically for given number of points. Both datasets consist of two dimensional points. The key difference is that while the Iris data is highly linearly separable, the other two datasets are non-separable in two dimensions. A subtle purpose of our study was to see if the optimizer can help the quantum neural network evolve a non-linear kernel to fit the Gaussian or Spirals datasets. 

\begin{table}[h]
    \centering
    \begin{tabular}{c|c|c}
    \toprule
      Dataset   & Dimensionality ($d$)  & Comments  \\
    \midrule
         Iris & 4 &  Reduced to binary classification problem  \\
         Gaussian & 2 & Two multivariate Gaussians drawn from different $\bm{\mu}$ and $\bm{\Sigma}$ \\ 

         Spirals & 2 & Spirals generated in two  different directions\\
    \bottomrule
    \end{tabular}
    \caption{Description and details of different datasets used in the study.}
    \label{tab:datasets_study}
\end{table}

Table~\ref{tab:datasets_study} shows a brief summary of the the datasets. For the Gaussian dataset we used $\bm{\mu}_1 = [2, 3]$, $\bm{\Sigma}_1 = [[10, 1], [1, 4]]$ and $\bm{\mu}_2 = [2, 3]$, $\bm{\Sigma}_2 = [[5, 2],[2,5]]$.  The spirals data was generated by sampling angles uniformly at random in clockwise and counter clockwise angles. The spirals in one direction were labeled as positive and the other direction was treated as negative. The relatively simple datasets considered in this study were necessitated in part due to the current inability of the quantum neural networks to scale to high dimensions and our goals of studying the optimization performance on simple controllable data. In future, we would like to extend our result to higher dimensional data as well.

\subsection{Algorithm Description}
\label{sec:sp_algdesc}

Algorithm~\ref{alg:rnn_opt} shows the optimization algorithm in more detail. Specifically, we look at the moving parts during some slice of training when at least a single meta-iteration has been completed. We assume that at that point, the replay buffer was in state $\mathcal{B}^T$. If during the previous meta-iteration we're able to find good parameter suggestions then $R > 1$ and the first condition becomes true. We build a seed parameter following Equation~\ref{eq:replay_buffer_update} and take the hidden state of LSTM from the sampled state returned by $s(\mathcal{B}^T)$. The cost history buffer $C^{hist}$ is initialized to be empty and the next meta-iteration is performed \emph{with the seeded parameters}. The parameters are updated using $LSTM\_UPDATE$ function that computes the new parameters as in Equation~\ref{eq:param-update-rule}. If during this iteration good parameters are found, they are added to the replay buffer. At the end of the training we perform an update on the meta-optimizer's parameters $\bm{\Phi}$ by computing loss function in Equation~\ref{eq:meta-optimizer}. If however we have not found a good candidate parameter then $R = 0$ and the other branch gets executed. In this, we simply set the seed to be the state at the end of last meta-iteration. The entire process is repeated until $|C(\bm{\theta})^{k+1} - C(\bm{\theta})^k| \leq \epsilon$ at the end of a meta-iteration.

\begin{algorithm}\caption{The Meta-Optimization Algorithm}
\label{alg:rnn_opt}
\begin{algorithmic}
\STATE {Initial State $s_{i}$}: [$\bm{\theta}^{i}, C(\bm{\theta}^{i}), \Delta C(\bm{\theta}^{i}), \bm{h}^{i})$]
\STATE {Hyperparameters}: [$\alpha,  T, \tau, R$]
\STATE {$W^{m}$}: [$w_0, w_1 \dots w_T$]

\STATE $\bm{\theta}^{pre} = \bm{\theta}^i$
\WHILE{not converged}
\IF{$R > 1$}
    \STATE $s(\mathcal{B}^T) \leftarrow$ SAMPLE\_FROM\_BUFFER()
    \STATE $\bm{\theta}^{pre} = \tau^t * \bm{\theta}^{T} + (1-\tau^t) * s(\mathcal{B}^{T})|_{\bm{\theta}^{T}}$ \COMMENT{$\bm{\theta}^{pre}$ are parameters before the start of new meta-iteration.} 
    \STATE $\bm{h}^{pre} = s(\mathcal{B}^{T})|_{\bm{h}^T}$ 
\ELSE  
    \STATE $\bm{\theta}^{pre} = \bm{\theta}^{T}$ \COMMENT{$\bm{\theta}^{T}$ are parameters at the end of the last meta-iteration}
     \STATE $\bm{h}^{pre} = \bm{h}^{T}$ 
\ENDIF
% \STATE $\bm{\theta}^{pre} = \theta$

\STATE {$C^{hist}$} $\leftarrow$ []
\STATE $\bm{\theta}^0 = \bm{\theta}^{pre}$
\STATE $\bm{h}^0 = \bm{h}^{pre}$
\FOR{$t = 1 \dots T$}
    \STATE {$\bm{\theta}^{t}, \bm{h}^{t} =$}  LSTM\_UPDATE($\bm{\theta}^{t-1},\bm{h}^{t-1}$)
    \STATE $c_{t} = C(\bm{\theta}^{t})$
    \STATE $C^{hist} = C^T \cup c_{t}$
    \IF{$c_{t} < c_{t-1}$}
        \STATE {ADD\_TO\_BUFFER($[\bm{\theta}^{t}, c_{t}, \Delta C(\bm{\theta}), \bm{h}^{t}]$)}
    \ENDIF
    % \STATE $s_{t-1}$ $\leftarrow$ \IIf{$|\mathcal{B}| > 1$}  \ElseIIF{$s_{t-1}$} \EndIIf  
\ENDFOR
    \STATE $\bm{\Phi}' \leftarrow $ {COMPUTE\_META\_LOSS($C^{hist}$, $W^{m}$)}
\ENDWHILE

\end{algorithmic}
\end{algorithm}

% \STATE {\bfseries Input:} Replay Buffer $B$, Weights $\bm{w}$, Meta-Horizon Size $T$, Previous state $p$
% \IF{p = $\phi$}
%     \STATE $\bm{\theta}$ = INIT\_NORMAL($q, L, blocks$)
%     \STATE $C(\bm{\theta})$ = 0 =  $\Delta C(\bm{\theta})$
%     \STATE $h^p, c^p$ = $\mathcal{N}(0, 1)$
%     \STATE $p$ = [$C(\bm{\theta}), \bm{\theta}, \Delta C(\bm{\theta}), h^p, c^p$]
% \ELSE
%     \IF{$B$ != $\phi$}
%         \STATE $bm{\theta}^s$ = SAMPLE($B$)
%         \STATE $\bm{\theta}^p$ = $\tau * \bm{\theta}^p$ + (1 - $\tau$) *  $bm{\theta}^s$
%         \STATE $p[1]$ = $\bm{\theta}^p$
%     \ENDIF
% \ENDIF

% \STATE Costs = []
% \WHILE{$t = 0 \dots T$}
%     \STATE $C(\bm{\theta}^p), \bm{\theta}, \Delta C(\bm{\theta}), h^p, c^p  \leftarrow p$ \\
%     \STATE $\bm{\theta}_{in}$ = $f_{in}([\bm{\theta}^p;\Delta C(\bm{\theta})]$
%     \STATE $\bm{\theta}^u, h^n, c^n$ = LSTM($\bm{\theta}_{in}, h^p, c^p$)
    
%     \STATE $\bm{\theta}^t = \bm{\theta}^p + \alpha * \sigma(\bm{\theta}^u)$
%     \IF{$C(\bm{\theta}^{t}) < C(\bm{\theta}^p)$}
%         \STATE $s \leftarrow [C(\bm{\theta}^{t}), \bm{\theta}^t, \Delta C(\bm{\theta}), h^n, c^n]$
%         \STATE $B \leftarrow s$
%     \ENDIF
%     \STATE $p \leftarrow [C(\bm{\theta}^{t}), \bm{\theta}^t, \Delta C(\bm{\theta}), h^n, c^n]$
%     \STATE Costs $\leftarrow C(\bm{\theta}^{t})$ 
% \ENDWHILE
% \STATE $L(\bm{\phi})$ = $\sum^{T} w$* Costs

% \STATE $\bm{\phi} \leftarrow \bm{\phi} - \eta * \nabla_{\bm{\phi}} L(\bm{\phi})$

\subsection{Effect of Initializing Distributions on Meta-Optmization Performance}
\label{ssec:ss-meta-distr}

We will now report the performance of our meta optimizer vis-à-vis classical gradient based methods that we have benchmarked against in this study. More specifically, we consider initializing the LSTM hidden states $\bm{h}^0$ with uniform distribution $\mathcal{U}(0, 1)$ and constant (zero) initialization in this ablation study. 

Figure~\ref{fig:ablation_hidden_state_init} shows the results of meta-optimizer performance on the Iris and the Gaussian datasets with the aforementioned initializing distributions. We observe that for linearly separable datasets with low number of points, a constant initialization results in the meta-optimizer searching over a vast space for a good descent direction. Consequently, the cost remains either same or divergent for a longer time than other gradient based optimizers. For more complex datasets like the Gaussian dataset, the performance is better but the meta optimizer gets stuck in far more inferior minima than competitive adaptive methods like Adam or RMSProp. Moreover, a constant initialization may lead to divergence if other hyperparameters are not selected carefully. 

There is a conventional wisdom in the current literature to select random parameters of an algorithm from a uniform distribution. We tested this wisdom with our meta optimizer on the same datasets. For the Iris dataset, we observe that the meta optimizer quickly gets stuck in a sub-optimal region and stays there for the rest of the training duration. For the Gaussian dataset, the optimizer performs a little better but again converges to a worse minima than the other gradient based optimizers. Keeping aside the fundamental differences in the methods, we can definitely conclude that a uniform initialization for hidden states can cause the meta optimizer to suggest parameters that converge to a sub-optimal minima.

\begin{figure*}[t]
    \centering
    \begin{subfigure}[t]{.35\textwidth}
     \centering
     \includegraphics[width=\textwidth]{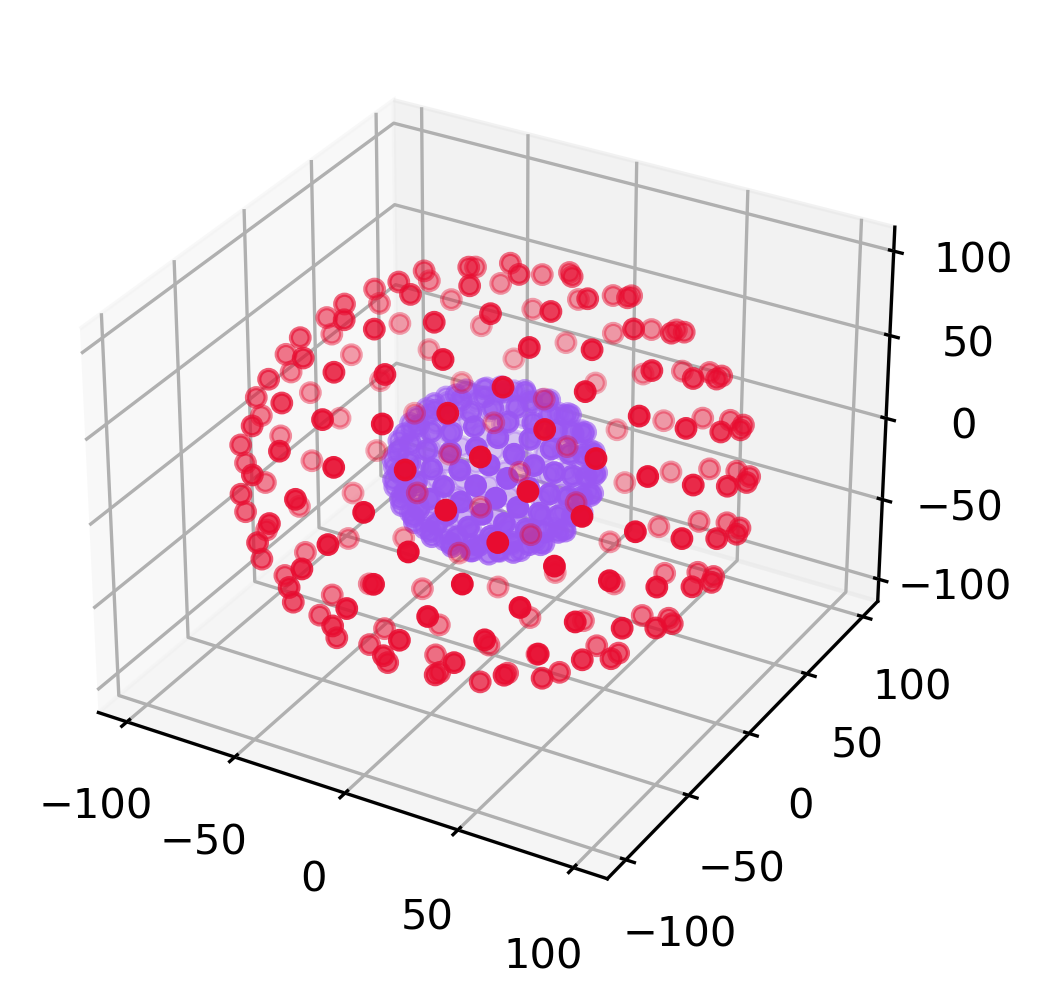}
    \caption{Spheres Dataset Visualization}
    \label{sfig:spheres_viz}
    \end{subfigure}
    
    \begin{subfigure}[t]{.7\textwidth}
     \centering
     \includegraphics[width=\textwidth, height=.25\textwidth]{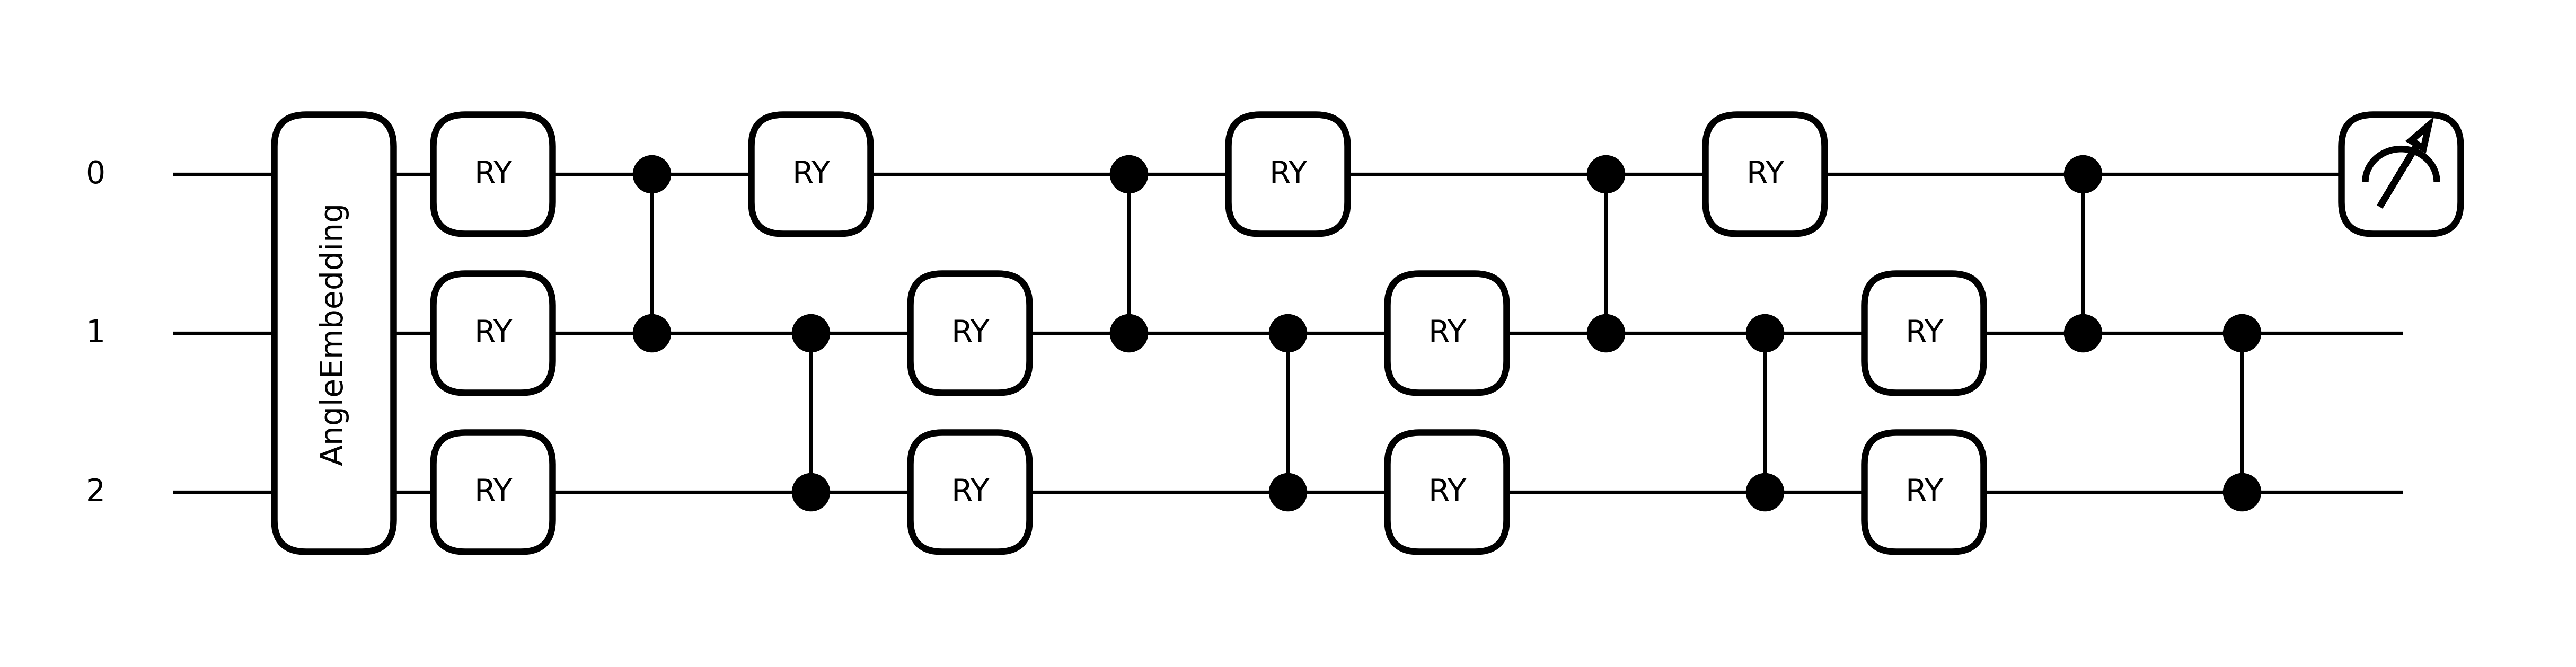}
    \caption{Quantum Circuit For Spheres Dataset}
    \label{sfig:qckt}
    \end{subfigure}

    \begin{subfigure}[t]{.35\textwidth}
     \centering
     \includegraphics[width=\textwidth]{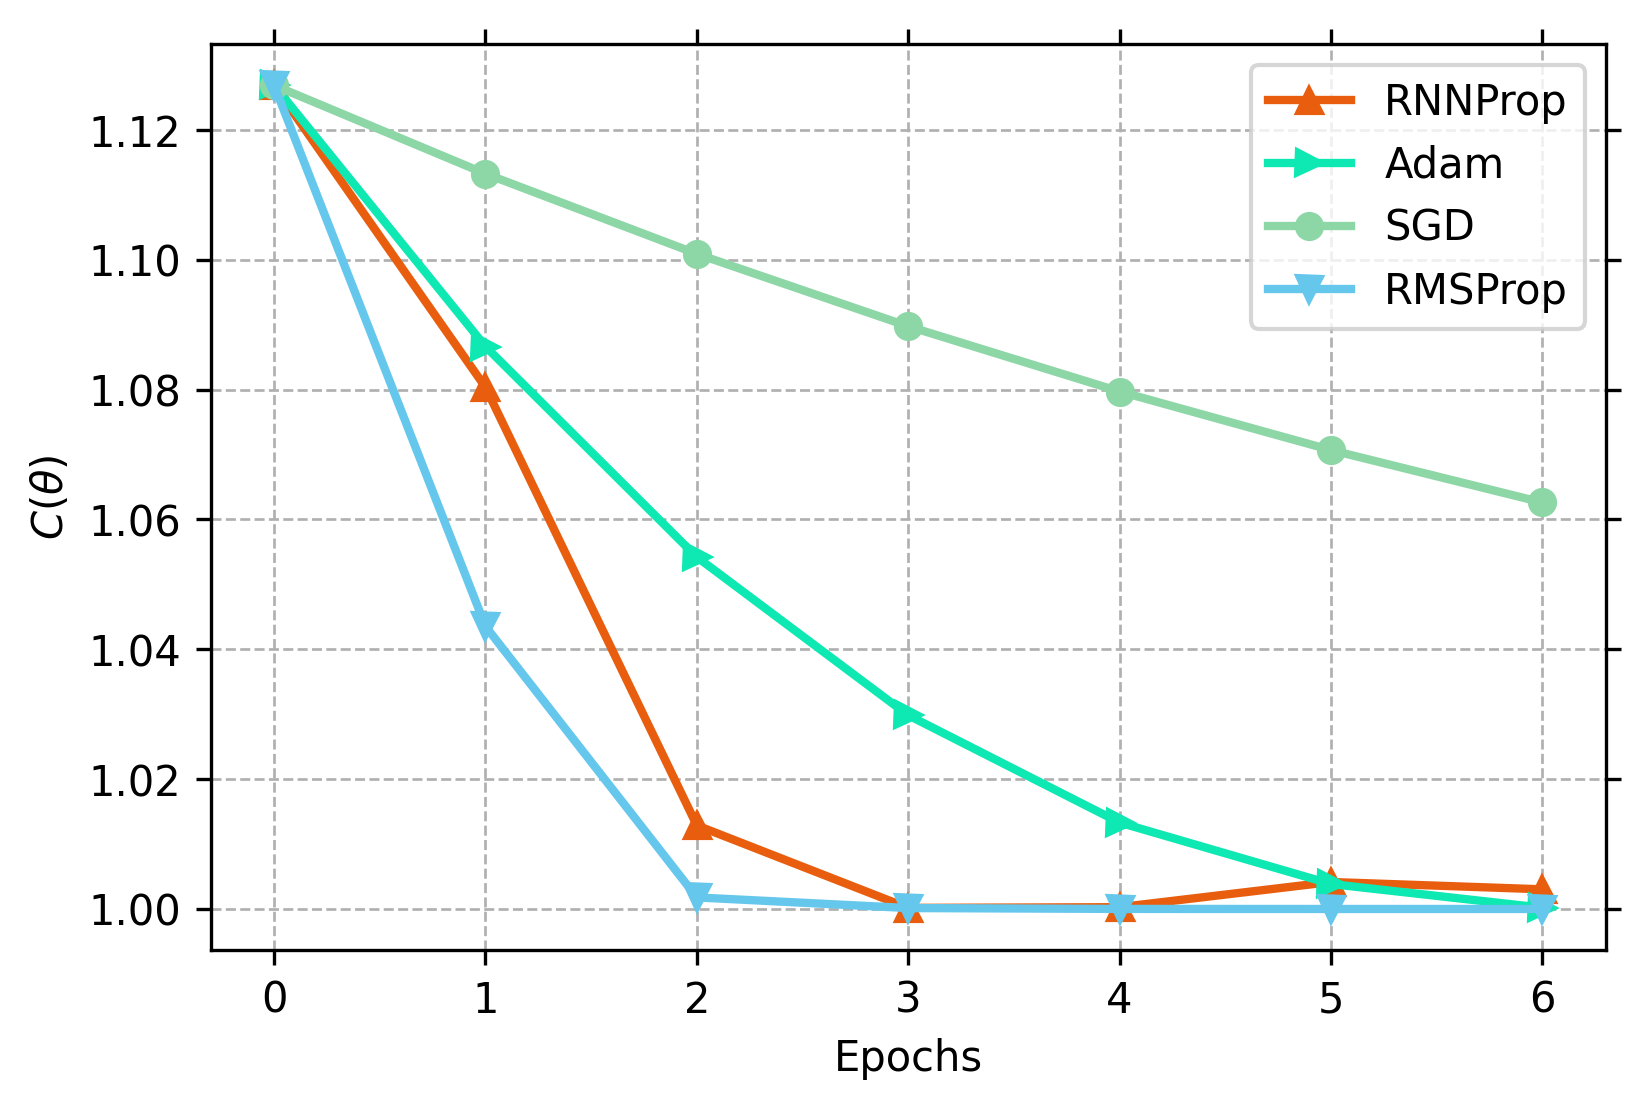}
    \caption{Optimization Results for Spheres dataset.}
    \label{sfig:spheres_opt_results}
    \end{subfigure}

    \caption{The spheres dataset and the quantum circuit used in our experiment. We embed the three dimensional point as rotational 
    angles of the RY gate. The circuit consists of four identical layers and the output is the expectation over the possible values of the first qubit in the eigenbasis of the Pauli-Z gate.}
    \label{fig:spheres_dataset}
\end{figure*}

\section{Experiments with Other Datasets}

We experimented with our algorithm on a more complex 3-dimensional dataset in which we generated 3-dimensional points representing two concentric spheres with one sphere having a significantly smaller radius than the other. The binary classification task is to predict if a given 3d point is on the outer or inner sphere. The dataset (\ref{sfig:spheres_viz}) and the circuit (\ref{sfig:qckt}) used are shown in Figure~\ref{fig:spheres_dataset}. The circuit consists of four layers with each layer consisting of parameterized RY gates which are entangled together using the CZ gates. 

We minimally changed the experimental setup and measured the convergence performance along with the time per epoch metric. We compare them with the performance exhibited by the other three optimizers considered in this work. The results are shown in Figure~\ref{sfig:spheres_opt_results}. We can observe that for this dataset and the circuit, our optimizer performs much better than the Adam and SGD optimizers.  In fact, our optimizer performs comparably to the RMSProp optimizer in terms of convergence performance. This illustrates that with the right circuit a gradient free method like ours can achieve similar performance minus the overhead of computing gradients via the parameter shift method.
