# Supplementary material for: Learning To Optimize Quantum Neural Network Without Gradients
Source: arXiv:2304.07442 source file (2023-04-15)
Supplement: Supplementary file 2 [file appendix.tex]

\section{The Meta Optimization Algorithm}
An overview of a single meta-iteration step is shown in Algorithm~\ref{alg:rnn_opt}.

\begin{algorithm}\caption{The Meta-Optimization Algorithm}
\label{alg:rnn_opt}
\begin{algorithmic}
\STATE {Initial State $s_{i}$}: [$\bm{\theta}^{i}, C(\bm{\theta}^{i}), \Delta C(\bm{\theta}^{i}), \bm{h}^{i})$]
\STATE {Hyperparameters}: [$\alpha,  T, \tau, R$]
\STATE {$W^{m}$}: [$w_0, w_1 \dots w_T$]

\STATE $\bm{\theta}^{pre} = \bm{\theta}^i$
\WHILE{not converged}
\IF{$R > 1$}
    \STATE $s(\mathcal{B}^T) \leftarrow$ SAMPLE\_FROM\_BUFFER()
    \STATE $\bm{\theta}^{pre} = \tau^t * \bm{\theta}^{T} + (1-\tau^t) * s(\mathcal{B}^{T})|_{\bm{\theta}^{T}}$ \COMMENT{$\bm{\theta}^{pre}$ are parameters before the start of new meta-iteration.} 
    \STATE $\bm{h}^{pre} = s(\mathcal{B}^{T})|_{\bm{h}^T}$ 
\ELSE  
    \STATE $\bm{\theta}^{pre} = \bm{\theta}^{T}$ \COMMENT{$\bm{\theta}^{T}$ are parameters at the end of the last meta-iteration}
     \STATE $\bm{h}^{pre} = \bm{h}^{T}$ 
\ENDIF
% \STATE $\bm{\theta}^{pre} = \theta$

\STATE {$C^{hist}$} $\leftarrow$ []
\STATE $\bm{\theta}^0 = \bm{\theta}^{pre}$
\STATE $\bm{h}^0 = \bm{h}^{pre}$
\FOR{$t = 1 \dots T$}
    \STATE {$\bm{\theta}^{t}, \bm{h}^{t} =$}  LSTM\_UPDATE($\bm{\theta}^{t-1},\bm{h}^{t-1}$)
    \STATE $c_{t} = C(\bm{\theta}^{t})$
    \STATE $C^{hist} = C^T \cup c_{t}$
    \IF{$c_{t} < c_{t-1}$}
        \STATE {ADD\_TO\_BUFFER($[\bm{\theta}^{t}, c_{t}, \Delta C(\bm{\theta}), \bm{h}^{t}]$)}
    \ENDIF
    % \STATE $s_{t-1}$ $\leftarrow$ \IIf{$|\mathcal{B}| > 1$}  \ElseIIF{$s_{t-1}$} \EndIIf  
\ENDFOR
    \STATE $\bm{\Phi}' \leftarrow $ {COMPUTE\_META\_LOSS($C^{hist}$, $W^{m}$)}
\ENDWHILE

\end{algorithmic}
\end{algorithm}

% \STATE {\bfseries Input:} Replay Buffer $B$, Weights $\bm{w}$, Meta-Horizon Size $T$, Previous state $p$
% \IF{p = $\phi$}
%     \STATE $\bm{\theta}$ = INIT\_NORMAL($q, L, blocks$)
%     \STATE $C(\bm{\theta})$ = 0 =  $\Delta C(\bm{\theta})$
%     \STATE $h^p, c^p$ = $\mathcal{N}(0, 1)$
%     \STATE $p$ = [$C(\bm{\theta}), \bm{\theta}, \Delta C(\bm{\theta}), h^p, c^p$]
% \ELSE
%     \IF{$B$ != $\phi$}
%         \STATE $bm{\theta}^s$ = SAMPLE($B$)
%         \STATE $\bm{\theta}^p$ = $\tau * \bm{\theta}^p$ + (1 - $\tau$) *  $bm{\theta}^s$
%         \STATE $p[1]$ = $\bm{\theta}^p$
%     \ENDIF
% \ENDIF

% \STATE Costs = []
% \WHILE{$t = 0 \dots T$}
%     \STATE $C(\bm{\theta}^p), \bm{\theta}, \Delta C(\bm{\theta}), h^p, c^p  \leftarrow p$ \\
%     \STATE $\bm{\theta}_{in}$ = $f_{in}([\bm{\theta}^p;\Delta C(\bm{\theta})]$
%     \STATE $\bm{\theta}^u, h^n, c^n$ = LSTM($\bm{\theta}_{in}, h^p, c^p$)
    
%     \STATE $\bm{\theta}^t = \bm{\theta}^p + \alpha * \sigma(\bm{\theta}^u)$
%     \IF{$C(\bm{\theta}^{t}) < C(\bm{\theta}^p)$}
%         \STATE $s \leftarrow [C(\bm{\theta}^{t}), \bm{\theta}^t, \Delta C(\bm{\theta}), h^n, c^n]$
%         \STATE $B \leftarrow s$
%     \ENDIF
%     \STATE $p \leftarrow [C(\bm{\theta}^{t}), \bm{\theta}^t, \Delta C(\bm{\theta}), h^n, c^n]$
%     \STATE Costs $\leftarrow C(\bm{\theta}^{t})$ 
% \ENDWHILE
% \STATE $L(\bm{\phi})$ = $\sum^{T} w$* Costs

% \STATE $\bm{\phi} \leftarrow \bm{\phi} - \eta * \nabla_{\bm{\phi}} L(\bm{\phi})$
